# Supplementary material for: Benchmarking of Quantum and Classical Computing in Large-Scale Dynamic Portfolio Optimization Under Market Frictions
Source: arXiv:2502.05226 source file (2025-02-06)
Supplement: Supplementary file 1 [file appendix.tex]

\subsection*{Proof of Lemma 2.1}
Portfolio value $\mathbf{1}^{\mathsf{T}}\mathbf{P}_t\mathbf{y}_t+c_t>0$ for $t=1,...,T$. Let $S_t=\mathbf{1}^{\mathsf{T}}\mathbf{P}_t\mathbf{y}_t+c_t$, so $S_1,...,S_T$ are positive and bounded. We let $S_{max}=max\{S_1,S_2,...,S_T\}>0$ and $S_{min}=min\{S_1,S_2,...,S_T\}>0$.
Consider the value of $\boldsymbol{\mu}_t^{\mathsf{T}}\mathbf{P}_t \mathbf{y}_t+rc_t$ for $t$ from $1$ to $T$.

Case 1: If all values of $\boldsymbol{\mu}_t^{\mathsf{T}}\mathbf{P}_t \mathbf{y}_t+rc_t$ are non-negative, let $\boldsymbol{\mu}_t^{\mathsf{T}}\mathbf{P}_t \mathbf{y}_t+rc_t=a_t$, we have
\begin{equation}\label{eq:positive_range}
    0\leq\frac{1}{S_{max}}\sum_{t=1}^Ta_t \leq \sum_{t=1}^T\frac{a_t}{S_t} \leq \frac{1}{S_{min}}\sum_{t=1}^Ta_t
\end{equation}
Let $A=\sum_{t=1}^Ta_t$. Consider $x \in [S_{min},S_{max}] \subset \mathbb{R}^1$ is a compact set. $f:[S_{min},S_{max}] \rightarrow \mathbb{R}^1, f(x)=\frac{A}{x}$. Since $f(x)$ is a continuous function, according to the Heine-Borel theorem, the codomain of $f(x)$ is a compact set, and $f(x) \in [\frac{A}{S_{max}},\frac{A}{S_{min}}]$ for any $x$ in domain, according to the Corollary of Cantor-Heine theorem. From \ref{eq:positive_range}, we know \text{portfolio return} in codomain of $f(x)$. 

Case 2: If all values of $\boldsymbol{\mu}_t^{\mathsf{T}}\mathbf{P}_t \mathbf{y}_t+rc_t$ are negative, let $\boldsymbol{\mu}_t^{\mathsf{T}}\mathbf{P}_t \mathbf{y}_t+rc_t=b_t$, we have
\begin{equation}\label{eq:negative_range}
    \frac{1}{S_{min}}\sum_{t=1}^Tb_t \leq \sum_{t=1}^T\frac{b_t}{S_t} \leq \frac{1}{S_{max}}\sum_{t=1}^Tb_t < 0
\end{equation}
Let $B=\sum_{t=1}^Tb_t$. Consider $x \in [S_{min},S_{max}] \subset \mathbb{R}^1$ is a compact set. $f:[S_{min},S_{max}] \rightarrow \mathbb{R}^1, f(x)=\frac{B}{x}$. Since $f(x)$ is a continuous function, according to the Heine-Borel theorem, the codomain of $f(x)$ is a compact set, and $f(x) \in [\frac{B}{S_{min}},\frac{B}{S_{max}}]$ for any $x$ in domain, according to the Corollary of Cantor-Heine theorem. From \ref{eq:negative_range}, we know \text{portfolio return} in codomain of $f(x)$. 

Hence, there exists $x_0 \in [S_{min},S_{max}]$ such that $f(x_0)$ = \text{portfolio return} if the signs of all $\boldsymbol{\mu}_t^{\mathsf{T}}\mathbf{P}_t \mathbf{y}_t+rc_t$ are the same. We can obtain
\begin{equation}
    \text{Portfolio return}=\frac{1}{x_0}\sum_{t=1}^T\Big(\boldsymbol{\mu}_t^{\mathsf{T}}\mathbf{P}_t\mathbf{y}_t+rc_t\Big)
\end{equation}

Case 3: If some values of $\boldsymbol{\mu}_t^{\mathsf{T}}\mathbf{P}_t\mathbf{y}_t + rc_t$ are non-negative and the others are negative, we divide them into two groups based on their signs. Without loss of generality, let's assume $\boldsymbol{\mu}_1^{\mathsf{T}}\mathbf{P}_1 \mathbf{y}_1+rc_1,...,\boldsymbol{\mu}_m^{\mathsf{T}}\mathbf{P}_m\mathbf{y}_m+rc_m$ are non-negative, and $\boldsymbol{\mu}_{m+1}^{\mathsf{T}}\mathbf{P}_{m+1} \mathbf{y}_{m+1}+rc_{m+1},...,\boldsymbol{\mu}_T^{\mathsf{T}}\mathbf{P}_T\mathbf{y}_T+rc_T$ are negative. Using the above notations $S_{max}$ and $S_{min}$. Let $\boldsymbol{\mu}_t^{\mathsf{T}}\mathbf{P}_t \mathbf{y}_t+rc_t=a_t\ge 0$ for $t = 1,...,m$, and $\boldsymbol{\mu}_t^{\mathsf{T}}\mathbf{P}_t \mathbf{y}_t+rc_t=b_t<0$ for $t = m+1,...,T$. Then we have 
\begin{equation}\label{eq:vary_range}
   \frac{1}{S_{max}}\sum_{t=1}^ma_t+\frac{1}{S_{min}}\sum_{t=m+1}^Tb_t\leq \sum_{t=1}^m\frac{a_t}{S_t}+\sum_{t=m+1}^T\frac{b_t}{S_t}\leq \frac{1}{S_{min}}\sum_{t=1}^ma_t+\frac{1}{S_{max}}\sum_{t=m+1}^Tb_t
\end{equation}
Consider $(x,y) \in [S_{min}, S_{max}] \times [S_{min}, S_{max}] \subset \mathbb{R}^2$ is a compact set. Let $A=\sum_{t=1}^ma_t\ge 0, B=\sum_{t=m+1}^Tb_t<0$, and $f:[S_{min}, S_{max}] \times [S_{min}, S_{max}] \rightarrow \mathbb{R}, f(x,y)=\frac{A}{x}+\frac{B}{y}$. It is easy to verify that $f(x,y)$ is a continuous function. The codomain of $f(x,y)$ is a compact set, and $f(x,y) \in \left[\frac{A}{S_{max}}+\frac{B}{S_{min}}, \frac{A}{S_{min}}+\frac{B}{S_{max}} \right]$ for any given $x,y$ in domain. Form \label{eq:vary_range}, we know portfolio return is in the codomain of $f(x,y)$. Therefore, there exists $(x_0,y_0) \in [S_{min}, S_{max}] \times [S_{min}, S_{max}] $ such that $f(x_0,y_0)=\text{portfolio return}$. 

Consider $g:\mathbb{R}^+ \rightarrow \mathbb{R}$,  $g(z)=\frac{A+B}{z}$. If $\frac{A}{S_{max}}+\frac{B}{S_{min}} > 0$, then $A+B$ must $>0$; if $\frac{A}{S_{min}}+\frac{B}{S_{max}} < 0$, then $A+B$ must $<0$. In both scenarios, solving $g(z)=f(x_0,y_0)$, we obtain $z=\frac{(A+B)x_0y_0}{Ay_0+Bx_0}\in\mathbb{R}^+$ as long as $Ay_0+Bx_0\neq 0$. Therefore, \text{portfolio return} can be expressed as
\begin{equation}
    \text{Portfolio return}=\frac{1}{z}\sum_{t=1}^T\Big(\boldsymbol{\mu}_t^{\mathsf{T}}\mathbf{P}_t\mathbf{y}_t+rc_t\Big)
\end{equation}
Given cases 1, 2 and 3, there exists a positive number $C'$ that satisfies
\begin{equation}
    \text{Portfolio return}=C'\sum_{t=1}^T\Big(\boldsymbol{\mu}_t^{\mathsf{T}}\mathbf{P}_t\mathbf{y}_t+rc_t\Big)
\end{equation}
On the other hand, because for each $t=1,...,T, \Sigma_t$ is a positive definite matrix, given a vector $\mathbf{P}_t \mathbf{y}_t \ (t=1,...,T)$, $(\mathbf{P}_t \mathbf{y}_t)^{\mathsf{T}}\Sigma_t(\mathbf{P}_t \mathbf{y}_t)>0$ (all signs are positive). We can use the same method which discussed above to prove that, there exists a positive number $C''$, which satisfies
\begin{equation}
    \text{Stocks covariance}=C''\sum_{t=1}^T(\mathbf{P}_t \mathbf{y}_t)^{\mathsf{T}}\Sigma_t(\mathbf{P}_t \mathbf{y}_t)
\end{equation}

\subsection{Quantum Algorithms}
The discrete nature of the Ising spin-glass formulation introduces combinatorial complexity, making it challenging to find the optimal solutions efficiently. Given the computational complexity of the problem, in this work, we explore a diverse rage of advanced optimization technique and hardware implementations to address the dynamic portfolio optimization problem in its discrete formulation.

\subsection*{Quantum Annealing} 
Adiabatic quantum optimization \citep{mcgeoch2022adiabatic} offers a promising strategy to tackle complex computational problems, and it is is formulated based on certain properties of quantum particle processes governed by the Schrödinger equation
\begin{align} \label{equation: Schrodinger}
    i\hbar \frac{d\ket{\phi(t)}}{dt}=\mathcal{H}(t)\ket{\phi(t)}
\end{align}
over the time interval $[0,\tau]$, where $\hbar$ is the reduced Planck constant, and $\mathcal{H}(t)$ is a time-varying Hermitian matrix representing the quantum system's Hamiltonian. In this approach, the solution to the optimization problem is encoded in the ground state, corresponding to the lowest eigenvalue of a quantum Hamiltonian, denoted as $\mathcal{H}_F$. 

According to the second postulate of quantum mechanics, a quantum system's dynamics are entirely determined by its Hamiltonian. By encoding the objective function to be minimized into the Hamiltonian of a quantum system, identifying the ground state of the Hamiltonian becomes equivalent to finding the set of decision variables that minimize the objective function.

The adiabatic evolution of the quantum system starts with its preparation in the ground state of a known Hamiltonian $\mathcal{H}_I$. Then, the system's Hamiltonian is slowly changed from $\mathcal{H}_I$ at $t=0$ to the final Hamiltonian $\mathcal{H}_F$ at $t=\tau$ through the time-varying function $s(t)$, which is a continuous adiabatic evolution path decreasing from $s(0) = 1$ to $s(\tau) = 0$. If $\tau$ is large enough and $\mathcal{H}_I$ and $\mathcal{H}_F$ do not commute, the quantum system will predominantly remain in the ground state during the evolution
\begin{align}
    \mathcal{H}(t)=s(t)\mathcal{H}_I+\big(1-s(t)\big)\mathcal{H}_F
\end{align}
Consequently, measuring the quantum state at $t=\tau$ will yield a solution to the optimization problem in the form of a bitstring representing an optimal configuration of binary decision variables that minimize the objective function encoded in $\mathcal{H}_F$. 
%这里V和E和前面表示C矩阵
The connectivity structure of the general objective function is represented by a graph $G = (V, E)$, where $V$ is the set of vertices and $E$ is the set of edges. D-Wave's approach involves finding a minor embedding of the graph $G$ onto a specialized hardware working graph $H$, often constructed as a Chimera graph. This mapping enables the utilization of the quantum annealer's hardware resources, which are organized according to the structure of graph $H$. 

D-Wave's quantum annealers can effectively translate our objective function into the language of the hardware's qubits and interactions. The quantum annealing algorithm employed by D-Wave incorporates the initial Hamiltonian $\mathcal{H}_I$ and the problem Hamiltonian $\mathcal{H}_F$. These Hamiltonians play a crucial role in defining the quantum annealing process.

The initial Hamiltonian $\mathcal{H}_I$ is defined as
\begin{align}
    \mathcal{H}_I=\sum_i \sigma_i^x
\end{align}
where $\sigma_i^x$ represents the Pauli-X operator acting on qubit $i$. This initial Hamiltonian is designed to ensure that the quantum system explores a broad solution space at the beginning of the annealing process.

The problem Hamiltonian $\mathcal{H}_F$ is formulated as
\begin{align}
    \mathcal{H}_F=\sum_i h_i \sigma_i^z + \sum_{i<j}J_{ij} \sigma_i^z \sigma_j^z
\end{align}
Here, $h_i$ represents the local fields, and $J_{ij}$ denotes the coupling strengths between qubits $i$ and $j$. These parameters are constrained to match the hardware's working graph.

The annealing process follows a predefined transition path, defined by a pair of envelope functions $A(s)$ and $B(s)$. The transition parameter $s(t): 0 \longrightarrow 1$ as $t: 0\longrightarrow \tau$ for a total transition time $\tau$. The function $s(t)$ is not strictly linear; it exhibits a "slowing down" around the middle of the transition, which enhances the quantum annealing process's efficiency and effectiveness.

Combining these components, the D-Wave quantum annealers implement the annealing Hamiltonian $\mathcal{H}(s)$ as a linear combination of the initial Hamiltonian $\mathcal{H}_I$ and the problem Hamiltonian $\mathcal{H}_F$:
\begin{align}
    \mathcal{H}(s)=A(s)\mathcal{H}_I+B(s)\mathcal{H}_F
\end{align}
This formulation allows the quantum system to traverse from the initial state defined by $\mathcal{H}_I$ to a final state that represents solutions to the optimization problem encoded in $\mathcal{H}_F$. The combination of the two Hamiltonians, along with the annealing path defined by $A(s)$ and $B(s)$, forms the basis of D-Wave's quantum annealing algorithm, providing a powerful approach for addressing optimization tasks using quantum techniques.
